# Supplementary material for: Lattice Dynamics of Energy Materials Investigated by Neutron Scattering
Source: arXiv:2504.17092 source file (2025-04-23)
Supplement: Supplementary file 1 [file appendix.tex]

% !TEX root = ../thesis.tex

\chapter{Bragg scattering (redux)} % *NOT* \OnePageChapter
\label{app:appendix}

\cref{sec:bragg_scattering} showed the microscopic, quantum mechanical derivation of Bragg scattering. Perhaps a more intuitive way to understand Bragg scattering is to consider elastic scattering of classical waves from classical atoms. For elastic scattering, we set the displacements to $\bm{u}(t)=0$ so that the atoms are frozen at their \emph{equilibrium} positions, $\hat{\bm{R}}_{ia}(t) = \bm{R}_i + \bm{\tau}_a$ (i.e. no thermal displacements). 

Assume an incoming classical wave with incoming amplitude $\psi_{in}(\bm{r}) = \psi_0 \exp(i\bm{k}_{in}\cdot\bm{r})$. The atoms in the region $ d\bm{r}'$ scatter neutrons into spherical waves with amplitude $\psi_{out}(\bm{r}) = \psi_0 \exp(i \bm{k}_{out} \cdot \bm{r}) b(\bm{r}') \rho(\bm{r}')  \exp( i k'|\bm{r}-\bm{r}'|)  / |\bm{r}-\bm{r}'| $ where $\rho(\bm{r}')$ is the density of scatterers at $\bm{r}'$, $b(\bm{r}')$ is the local scattering amplitude at $\bm{r}'$, and $\bm{r}$ is where we detect the scattered wave. By definition, the scattered wavevector $\bm{k}_{out}$ is parallel to $|\bm{r}'-\bm{r}|$ and $k_{out} | \bm{r}-\bm{r}'| = \bm{k}_{out} \cdot (\bm{r}-\bm{r}') $ (see \cref{fig:classical_scattering_diagram}). 

The net amplitude at the detector is, in general, the sum of all spherical waves scattered from every point in the sample: $\psi(\bm{r}) = \int  [ \psi_{in}(\bm{r}') + \psi_{out}(\bm{r}')] d\bm{r}' $. Usually the incoming wave is a beam of plane waves and the incoming waves that aren't scattered pass straight through the sample. The unscattered waves would saturate a detector, providing useless data, so we usually don't measure the transmitted part of the beam. Rather, we place a beam stop in the beam path on the down-stream side of the sample to collect all the unscattered particles, and look at different scattering angles instead. Then we can write the scattered intensity as
\begin{equation}\begin{split}
    I(\bm{r}) = \left| \psi_0 \frac{\exp(i\bm{k}_{out}\cdot \bm{r}) }{r'} \int \frac{b(\bm{r}') \exp(i (\bm{k}_{in}-\bm{k}_{out}) \cdot \bm{r}' ) \rho(\bm{r}')}{|\bm{r}-\bm{r}'|} \right|^2 .
\end{split}\end{equation}

\begin{figure}[t!]
    \centering
    \includegraphics[width=0.8\linewidth]{appendix/scattering_diagram.png}
    \caption{Scattering diagram for classical waves from classical matter. The magenta blob is the matter.}
    \label{fig:classical_scattering_diagram}
\end{figure}

We define $\bm{Q} \equiv \bm{k}_{in} - \bm{k}_{out}$, i.e the momentum transferred from the neutron into the sample. Usually the distance to the detectors, $|r|\sim$m, is much larger than the sample size, $|r'|\sim $mm. Then $|\bm{r}-\bm{r}'| \approx |r|$ (see \cref{fig:classical_scattering_diagram}). We assume the matter is a classical assembly of particles in a static, crystalline arrangement, so that $b(\bm{r})\rho(\bm{r}) = \sum_{ia} b_a \delta(\bm{r}-(\bm{R}_i + \bm{\tau}_a))$. Then
\begin{equation}\begin{split}
    I(\bm{r}) & \approx  \frac{|\psi_0|^2}{r^2} \left| \sum_{ia} \exp(i \bm{Q} \cdot ( \bm{R}_i + \bm{\tau}_a)) \right|^2 \\
    & = \frac{|\psi_0|^2}{r^2} \left| \left(  \sum_{i} \exp(i \bm{Q} \cdot \bm{R}_i ) \right) \left( \sum_{a} b_a \exp(i\bm{Q}\cdot\bm{\tau}_a) \right)  \right|^2
\end{split}\end{equation}
The phase at the detector depends on the distance from the scattering volume, $\bm{r}'$, to the detector at $\bm{r}$. But since the crystal is ordered, we can separate the coordinates $\bm{r}'$ into the coordinates of the unitcell origins and the coordinates of atoms in the unitcell relative to the unitcell origin. We can then separate the amplitude into the two contributions: the scattering from the arrangement of unitcells and the scattering from the atoms within the unitcells. 

The first term in parentheses is the total amplitude for scattering from all of the unitcell origins. For a truly infinite crystal, the sum over unitcells, $\sim \sum_{\bm{R}} \exp(i\bm{Q}\cdot\bm{R})$, becomes a $\delta$-function because, when the momentum transfer is equal to reciprocal lattice vector, $\bm{Q} 
= \bm{G}$, $\exp(i\bm{G}\cdot\bm{R}) = \exp( i 2\pi n) = 1$ and $\sum_i = N$. I.e. the amplitude of the wave scattered from every unitcell has the same phase at the detector. For a non-reciprocal lattice vector, $\bm{Q}\cdot\bm{R} \neq 2\pi n$ in general and the phases at the detector vary rapidly between waves from different unitcells in the crystal. In the limit of an infinite sample, the phases all interfere to cancel exactly. Thus, we only see intensity when we measure momentum transfer such that scattering from all unitcells interferes constructively. For a finite crystal, the different phases don't cancel exactly, but the intensity is still very sharply peaked near $\bm{Q} = \bm{G}$. Still, real samples are usually so large ($N \sim 10^{23}$) that the limit $N\rightarrow \infty$ is a reasonable assumption. Then
\begin{equation}\begin{split}
    I(\bm{r}) & = N^2 \frac{|\psi_0|^2}{r^2} \delta(\bm{Q}-\bm{G}) \left| \sum_{a} b_a \exp(i\bm{Q}\cdot\bm{\tau}_a) \right|^2
    \label{eq:intensity_appendix}
\end{split}\end{equation}
The other part of the intensity in \cref{eq:intensity_appendix} is the scattering from the basis atoms themselves. Since the phase depends on the distance from sample to detector, the phase depends on the coordinates of atoms in the unitcell.

Aside from the absence of the Debye-Waller factor (DWF), \cref{eq:intensity_appendix} is proportional to \cref{eq:elastic_cross_section}. The cross section can be recovered by multiplying the intensity by the area of the detector voxel, $r^2 d\Omega$, at the coordinate $\bm{r}$. The cross section is this quantity divided by the subtended angle, $d\Omega$, and the incident intensity, $|\psi_0|^2$:
\begin{equation}\begin{split}
    \left( \frac{d\sigma} {d\Omega}\right)_{el} & =  \frac{I(\bm{r}) r^2 d\Omega}{d\Omega} \\
    & = N^2 \delta(\bm{Q}-\bm{G}) \left|  \sum_{a} b_a \exp(i\bm{Q}\cdot\bm{\tau}_a) \right|^2 . 
\end{split}\end{equation}

\begin{comment}
\begin{figure}[t!]
    \centering
    \includegraphics[width=0.8\linewidth]{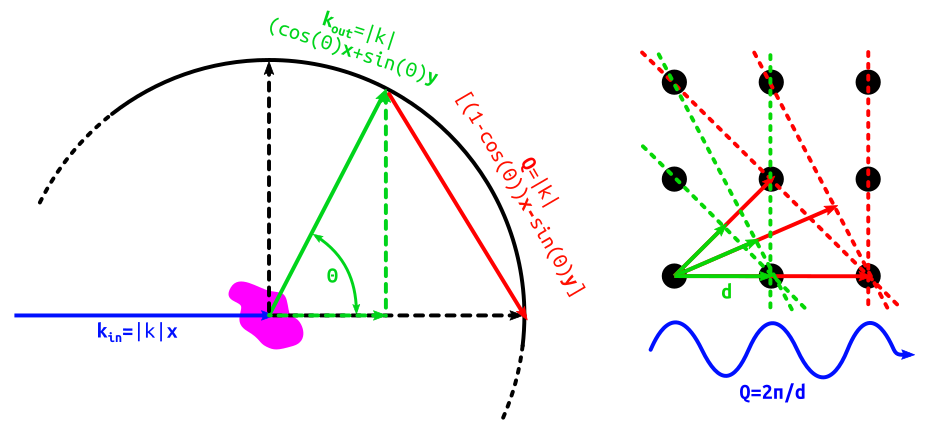}
    \caption{The momentum transfer into the sample, $\bm{Q}$, as a function of scattering angle for elastic scattering. The magenta blob is the sample. Assume $\bm{k}_{in} = k\hat{\bm{x}}$. For elastic scattering, $|\bm{k}_{in}| = |\bm{k}_{out}| = k$. Then $\bm{Q}=k [ \hat{\bm{x}} (1-\cos \theta) - \hat{\bm{y}} \sin\theta ]$. The right panel shows various $d$-spacings, i.e. the distance between lattice planes (the dashed lines). The $d$-spacings are the lengths of the vectors.}
    \label{fig:elastic_scattering_diagram}
\end{figure}
\end{comment}

The classical derivation shows that, up to the DWF, the Bragg intensity is due to interference-scattering from all of the static localized scattering centers in the crystal. Since the crystal is periodic, we only have to sum over a single unitcell. The phase is the same from unitcell-to-unitcell since $\exp( i\bm{G}\cdot\bm{R}) = \exp(i2\pi n) = 1$. The same intuition applies to \cref{eq:elastic_cross_section} with the nuance that the DWF factor lowers the amplitude for scattering from a given atom. The DWF essentially describes the thermal fluctuations around the mean and, for larger fluctuations, the atom spends less time near the equilibrium positions and the amplitude for scattering from the mean positions is reduced. 

%Suppose a scattering geometry like in \cref{fig:elastic_scattering_diagram}. Since only elastic scattering occurs, $|\bm{k}_{in}| = |\bm{k}_{out}| \equiv k$. As a function of scattering angle, $\bm{Q} = k [ \hat{\bm{x}} (1-\cos \theta) - \hat{\bm{y}} \sin\theta ]$. For an \emph{infinite} crystal
